# Supplementary material for: Nonlinear bias toward complex contagion in uncertain transmission settings
Source: arXiv:2302.13358 ancillary file (2023-12-30)
Supplement: Supplementary file 1 [file supporting_information.pdf]

# Supporting Information

## Nonlinear bias toward complex contagion in uncertain transmission settings

Guillaume St-Onge[1], Laurent Hébert-Dufresne[2,3,4], and Antoine Allard[2,4,5]

[1] *Laboratory for the Modeling of Biological and Socio-technical Systems, Northeastern University, Boston, MA, USA*
[2] *Vermont Complex Systems Center, University of Vermont, Burlington, VT 05401, USA*
[3] *Department of Computer Science, University of Vermont, Burlington, VT 05401, USA*
[4] *Département de physique, de génie physique et d'optique, Université Laval, Québec, QC G1V 0A6, Canada*
[5] *Centre interdisciplinaire en modélisation mathématique, Université Laval, Québec, QC G1V 0A6, Canada*

## 1 Time evolution: additional case studies

In this section, we show additional experiments for the temporal evolution of the effective transmission rate and the associated prevalence in the SIS and SIR model, similar to Fig. 2 in the main text.

In Fig. S1, we use the exact same conditions as for Fig. 2 in the main text, but we show the temporal evolution of the effective transmission rate for the SIR model instead in panel (a). We also include the critical effective transmission rate (obtained from Eq. (10), even though the SIS model is assumed) and its predictions for the prevalence. We see that the critical effective transmission rate is not too far from the eigenvector (EV) approximation.

In Fig. S2, we reduce the number of groups to which a node belongs and increased the scaling of the transmission rate distribution to remain in the supercritical regime. One thing we note is that the critical effective rate approximation is worse to predict the temporal evolution of the system; the eigenvector approximation remains accurate in the early stage of the outbreak.

In Fig. S3, we use Poisson distributions for the memberships and the group sizes. We see that the results are not too different from Fig. S1. Finally, in Fig. S4 and S5, we used a lognormal and a Fréchet distribution respectively for the group transmission rate.

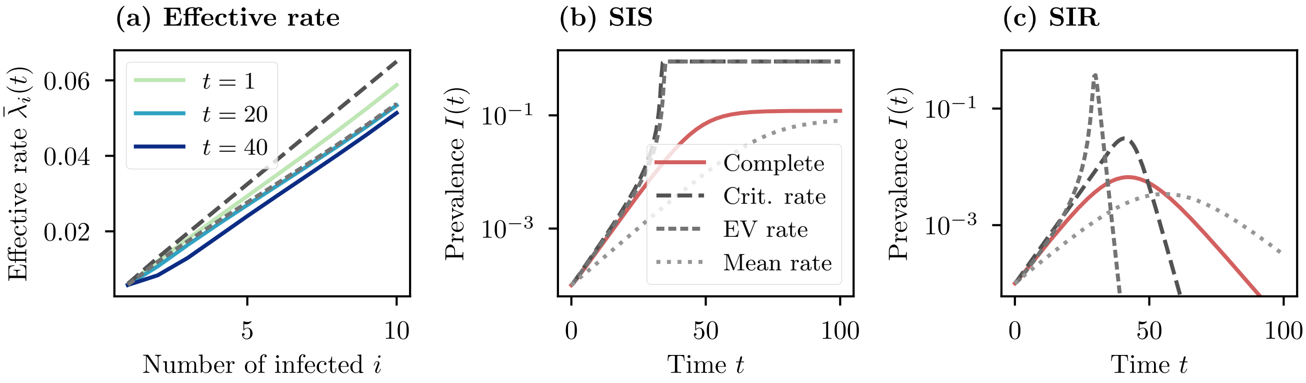


**Figure S1**: Temporal evolution of the effective transmission rate and its impact on the prevalence of the SIS and SIR dynamics. We use the same network as in Fig. 1(b) and (c). **(a)** The solid lines correspond to the exact effective transmission rate [Eq. (5)] measured at different times —here for the SIR model only. The large dashed line shows the critical effective transmission rate [Eq. (10)], the small dashed line shows the eigenvector (EV) approximation of Eq. (6). **(b)-(c)** The solid and dashed lines correspond to the numerical integration of the complete or coarse-grained dynamical system using different approximations for $\bar{\lambda}_i$.

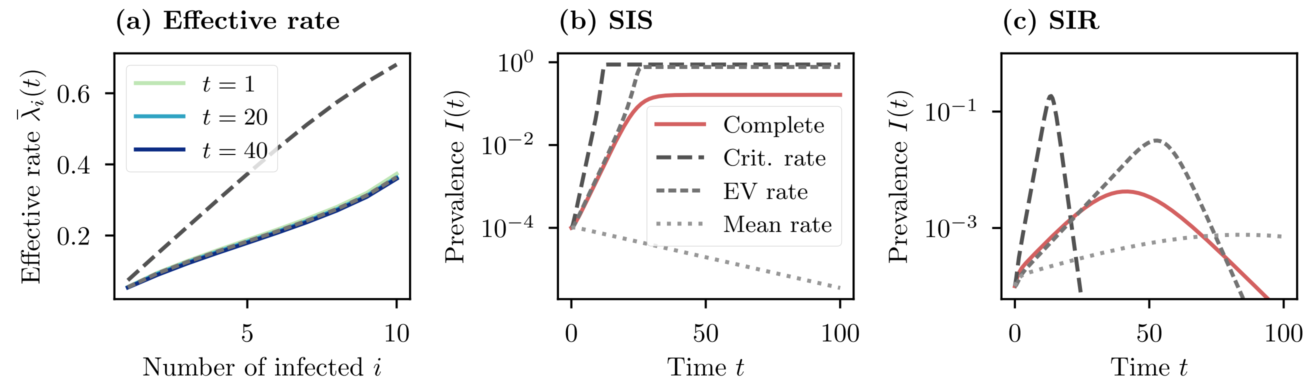


**Figure S2**: We use $q_m = \delta_{m,2}$, $p_n = \delta_{n,10}$, a discretized Weibull distribution with $\nu = 1$, $\mu = 6 \times 10^{-2}$ ($\mu = 7.5 \times 10^{-2}$ for the SIR model), and 500 points on the interval $\lambda \in [10^{-4}, 1]$.

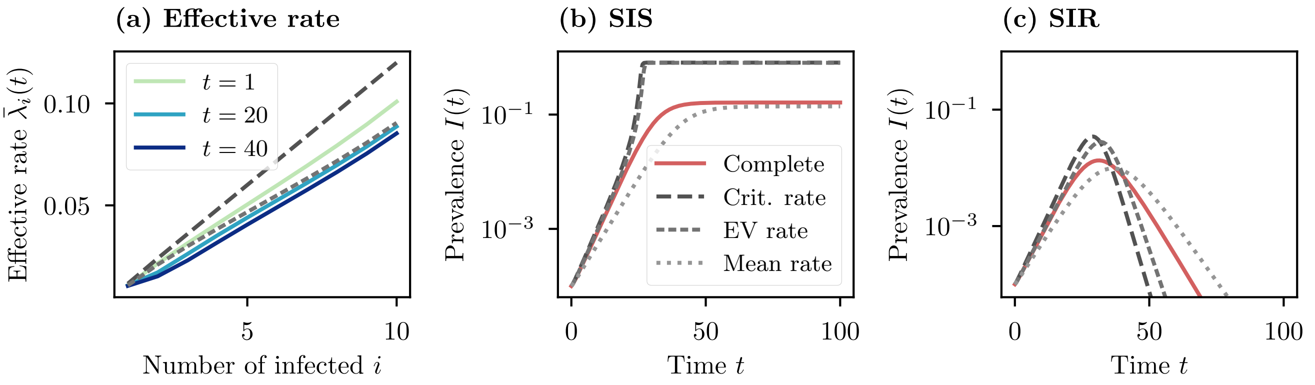


**Figure S3**: We use $q_m \sim \langle m \rangle^m e^{-\langle m \rangle}/m!$, $p_n =\sim \langle n \rangle^n e^{-\langle n \rangle}/n!$, with $\langle m \rangle = 20$ and $\langle n \rangle = 5$. We use a discretized Weibull distribution with $\nu = 1$, $\mu = 1.2 \times 10^{-2}$, and 500 points on the interval $\lambda \in [10^{-4}, 0.5]$.

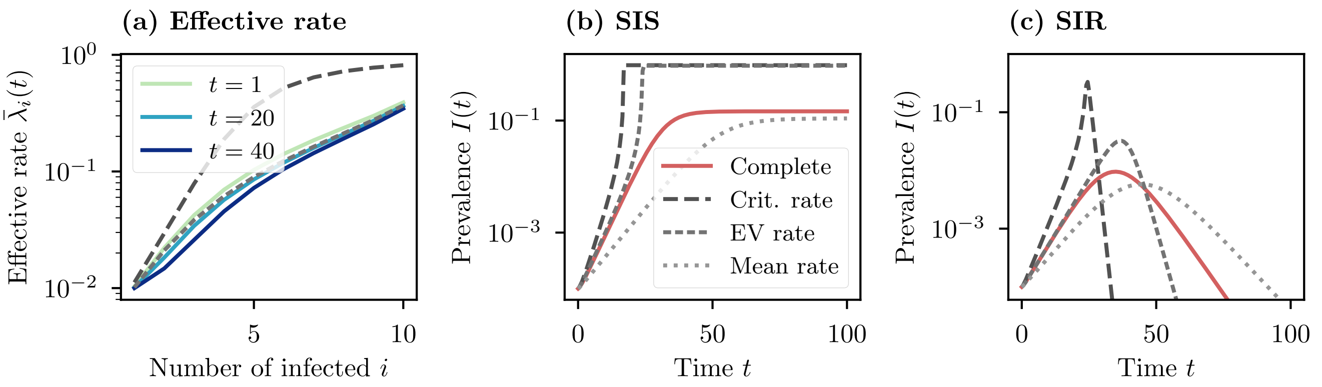


**Figure S4**: We use $q_m \sim \langle m \rangle^m e^{-\langle m \rangle}/m!$, $p_n =\sim \langle n \rangle^n e^{-\langle n \rangle}/n!$, with $\langle m \rangle = 20$ and $\langle n \rangle = 5$. We use a discretized lognormal distribution with $\nu = 1$, $\mu = 4 \times 10^{-3}$, and 500 points on the interval $\lambda \in [10^{-4}, 1]$.

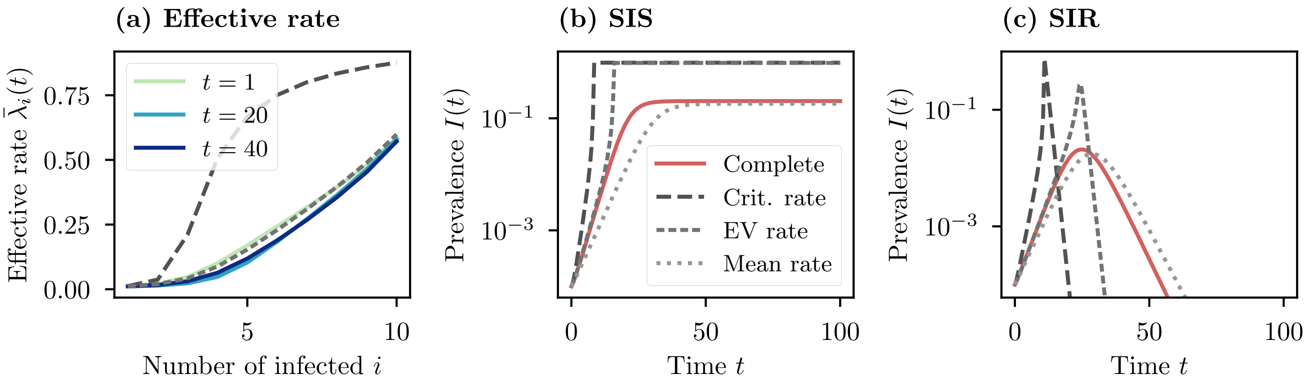


**Figure S5**: We use $q_m \sim \langle m \rangle^m e^{-\langle m \rangle}/m!$, $p_n =\sim \langle n \rangle^n e^{-\langle n \rangle}/n!$, with $\langle m \rangle = 20$ and $\langle n \rangle = 5$. We use a discretized Fréchet distribution with $\nu = 0.5$, $\mu = 7 \times 10^{-3}$, and 500 points on the interval $\lambda \in [10^{-4}, 1]$.

## 2 Nonlinear bias toward complex contagion

Figure 5 of the main text illustrates how the inference of simple contagion processes on weighted hypergraphs is biased toward nonlinear complex contagion if the group transmission heterogeneity is ignored. In this section, we detail the properties of the real hypergraphs we used and show that our results are robust to changing the nonlinear contagion model.

### 2.1 Properties of the hypergraphs

In Fig. 5 in the main text, we use hypergraphs constructed from data. In Table S1, we compile some statistics of the structure of the hypergraphs constructed. For instance, we see that the coauthorship hypergraph possess a very heterogeneous membership distribution, but a more homogeneous group size distribution.

**Table S1**: Structural properties of the hypergraphs used in Fig. 5 in the main text.

| | Group size | | | Membership | | |
|---|---|---|---|---|---|---|
| **Dataset** | $\langle n \rangle$ | $\sigma_n$ | $n_{\max}$ | $\langle m \rangle$ | $\sigma_m$ | $m_{\max}$ |
| Coauthorship | 3.84 | 1.73 | 25 | 4.47 | 21.00 | 1399 |
| High-school contacts | 2.32 | 0.53 | 5 | 55.63 | 27.06 | 148 |
| Email | 3.56 | 3.40 | 40 | 88.96 | 116.35 | 918 |

For the high-school contacts and the email dataset, we also have their weight distributions in Fig. S6, extracted from the repeated group interactions.

### 2.2 Another nonlinear contagion model

In the main text, we limit our analysis to infection rate of the form $\beta i^\alpha$ to show that superlinear contagion better describes the sequence of states when the underlying weights are ignored. However, other forms of nonlinear contagion can be used. In Fig. S7, we use the infection rate $\beta i \exp(i\alpha)$, which is the form we would recover for a lognormal distribution of group transmission. For both the high-school contact and email weighted hypergraphs, we see that superlinear contagion still better describes the time series.

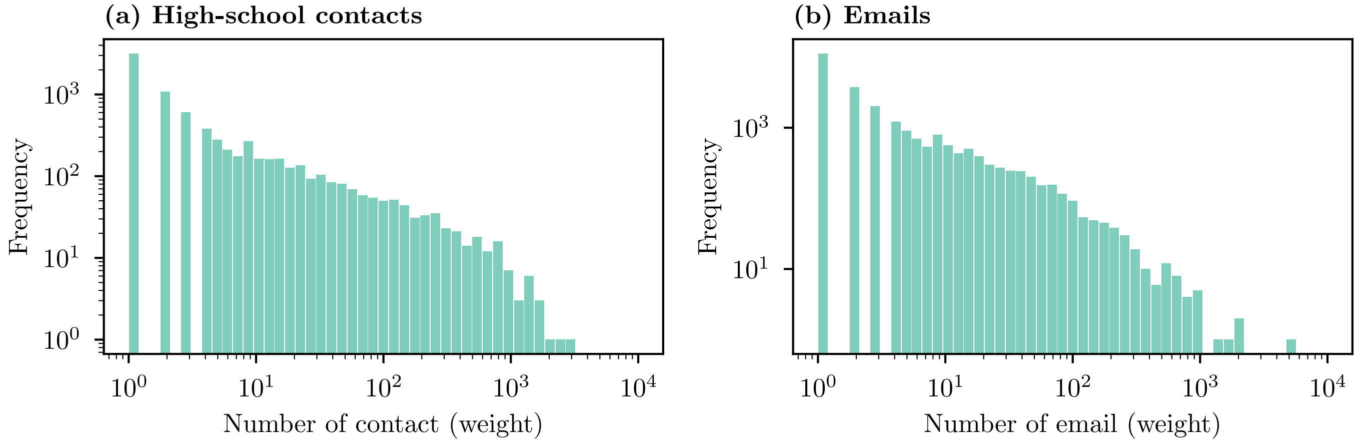


**Figure S6**: Distribution of the weights in the real hypergraphs used for the Bayesian inference experiments. (a) For the high-school contact patterns, for a given group of individuals, we associate the number of times these individuals interacted in group as the weight. (b) For the email dataset, we associate the number of times a same group of individuals were in an email as the weight for the group.

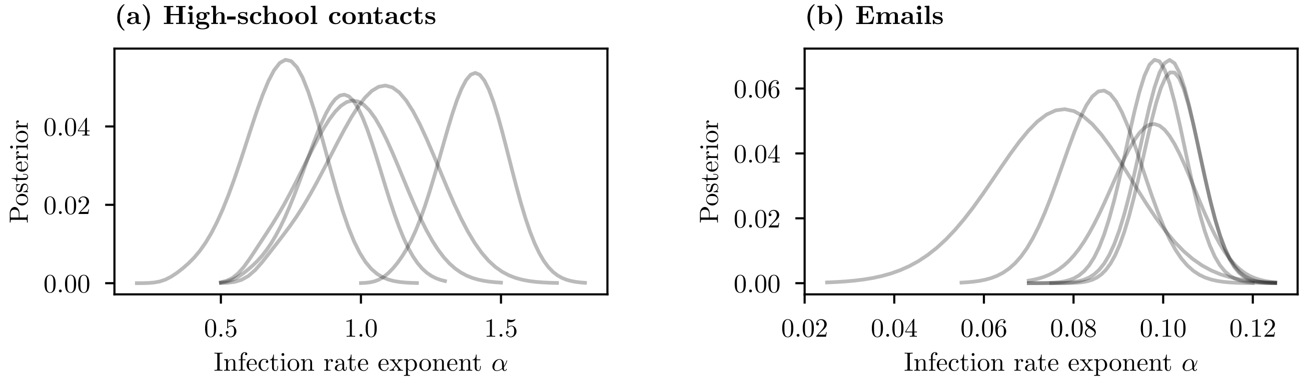


**Figure S7**: We use the same procedure as in Fig. 5 in the main text, but we instead use the superlinear infection rate $\beta i \exp(\alpha i)$.
